# Supplementary material for: Relative-error testing of conjunctions and decision lists
Source: arXiv:2504.08987 source file (2025-04-11)
Supplement: Supplementary file 1 [file DL-Conj-Appendix.tex]

%


%

%
%
%
%
%
%
%
%
%
%
      %
      %
       %
       %
%
%
%
       %
       %
        %
    %
%
%
%
%
%

%
%
%
       %
       %
        %
       %
%

%
%

%

    
